# Supplementary material for: Long-range model for electronic pseudospin-nuclear-spin coupling and two-stage ordering in TmVO$_4$
Source: arXiv:2507.16619 source file (2026-11-02)
Supplement: Supplementary file 1 [file Supplementary.tex]

\documentclass[aps,prb,onecolumn,superscriptaddress,notitlepage,showpacs,floatfix]{revtex4-2}
\usepackage{graphicx}
\usepackage{physics}
\usepackage{amsmath}
\usepackage{wasysym}
\usepackage{graphicx}
\usepackage{gensymb}
\usepackage{braket}
\usepackage{natbib}
\usepackage{comment}
\usepackage{physics}
\usepackage{color}
\usepackage{multirow}
\usepackage{array}
\usepackage[colorlinks=true,citecolor=blue,linkcolor=magenta, breaklinks=true]{hyperref}

\usepackage{subcaption}
\captionsetup{justification=raggedright,singlelinecheck=false}

\begin{document}

\title{Supplemental Material: Two-Stage Ordering and Elastocaloric Effect in TmVO$_4$}

\begin{abstract}
	We here provide supplemental explanations on the following topics in relation to the main text: (I) Mapping TmVO\(_4\) to an Infinite‐Range Transverse‐Field Ising Model, (II) Origin and expression of two combinatorial factors, $d(m)$ and $d(s_t)$, (III) Mean field analysis with transverse field ($h_x$), (IV) Finite-size scaling of the excitation gap near the critical point. 
\end{abstract}

\author{Sayan Ghosh}
\affiliation{S.N. Bose National Centre for Basic Sciences, Kolkata 700098, India.}
\author{Anirudha Menon}
\affiliation{Department of Physics, University of California Davis, Davis, California 95616, USA}
\affiliation{Centre for Theoretical and Computational Physics, National Yang Ming Chiao Tung University, Hsinchu City, Taiwan}
\author{Manoranjan Kumar}
\email{manoranjan.kumar@bose.res.in}
\affiliation{S.N. Bose National Centre for Basic Sciences, Kolkata 700098, India.}
\author{Rajiv R. P. Singh}
\email{rrpsing@ucdavis.edu}
\affiliation{Department of Physics, University of California Davis, Davis, California 95616, USA}

\date{\today}
\maketitle

\section{\label{SM1}Mapping TmVO\(_4\) to an Infinite‐Range Transverse‐Field Ising Model}

The low‐temperature physics of TmVO\(_4\) is governed by a well isolated $E_g$ crystal‐field doublet (separated by \(\sim54\)\,cm\(^{-1}\approx77\)\,K from the first excited level)\ \cite{knoll1971absorption}.  Below the cooperative Jahn–Teller transition at \(T_Q\approx2.2\)\,K, a spontaneous ferroquadrupolar \(B_{2g}\) order sets in, accompanied by a \(B_{2g}\) lattice distortion.  One can show that the quadrupole–strain coupling and the resulting phonon‐mediated interactions yield an effective all‑to‑all (\(1/N\)) “quadrupole–quadrupole” Hamiltonian, which in the pseudospin‑1/2 basis directly maps onto an infinite‐range Ising model.

Starting from the strain Hamiltonian shown in the supplementary of ref.\cite{massat2022field,zic_thesis,zic2025electro}:
\begin{equation}
  \hat H_s \;=\;
    \sum_{i} V_s\,\varepsilon_{B_{2g}}\,\hat P_{xy}(i)
    \;+\;\frac{C_{66}}{2}\,\varepsilon_{B_{2g}}^2
  \quad,\qquad
  \hat P_{xy}= \hat J_x\hat J_y + \hat J_y\hat J_x
  \label{eq:strain}
\end{equation}
minimization with respect to the static strain \(\varepsilon_{B_{2g}}\) produces a long‐range coupling
\begin{equation}
  \hat H_s^{(\mathrm{eff})}
    = -\,\frac{V_s^2}{2\,C_{66}}\;\sum_{i,j}\,\hat P_{xy}(i)\,\hat P_{xy}(j)
\,. \label{eq:massat_eff}
\end{equation}
A similar \(1/N\) coupling arises from integrating out the acoustic phonon modes (see refs. \cite{gehring1973cooperative,maharaj2017transverse}).  Since the lowest $E_g$ doublet can be treated as an effective pseudospin \(S=1/2\), one defines the Pauli operators-
\[
   \hat P_{xy}\;\to\; \hat S^z
   \,,\quad
   \hat O_{2}^2\,=\,\hat J_x^2-\hat J_y^2\;\to\;\hat S^y
   \,,\quad
   \hat J_z\;\to\;\hat S^x
\]
and the conjugate fields are respectively \(B_{2g}\) strain \(\varepsilon_{B_{2g}}\), \(B_{1g}\) strain \(\varepsilon_{B_{1g}}\), and magnetic field along the \(c\) axis \(H_z\)\ \cite{maharaj2017transverse}. We incorporate the nuclear coupling to the electronic degrees of freedom, in the form of a local nuclear spin $I^z_i$, and the resulting total Hamiltonian is given as follows :

\begin{equation}\label{eq:H}
\begin{split}
H=-\frac{2J_z}{N}\Bigl(\sum_{i}S_{i}^{z}\Bigr)^{2}
+2h_{y}\sum_{i}S_{i}^{y}
+2h_{x}\sum_{i}S_{i}^{x}
+4A\sum_{i}I_{i}^{z}(\frac{1}{N}\sum_jS_{j}^{x}),
\end{split}
\end{equation}
where:
\begin{itemize}
  \item \(\displaystyle J_z=\frac{V_s^2}{2\,C_{66}}\) is the effective infinite‐range quadrupolar coupling;
  \item \(h_x\propto H_z\) is the transverse magnetic field;
  \item \(h_y\propto\varepsilon_{B_{1g}}\) is the strain field;
  \item \(A\) is the nuclear hyperfine coupling.
\end{itemize}

Due to the long-range nature of the model we can write the model Hamiltonian in terms of a large total spin $\vec{S}_t=\sum_i \vec{S}_i$. In the infinite-range model, we treat the nuclear spins by a mean-field treatment, coupling each nuclear spin to the average electronic spin operator. Thus, the nuclear operator takes the form $I_t^z = \sum_i I_i^z$, which leads to an effective coupling of the type $H_A = \frac{4A}{N}I_t^zS_t^x$, where $S_t^x = \sum_i S_i^x$ is the total electronic spin along $x$.

%%%%%%%%%%%%%%%%%%%%%%%%%%%%%%%%%%%%%%%%%%%%%%%%%%%%%%%%%%%%%%%%%%%%%%%
\section{\label{SM2}Origin and mathematical expression for combinatorial factors}
The infinite-range model possesses a large number of symmetries. Since the Hamiltonian depends only on the three operators \( S^z_t, S^x_t, S^y_t \) and they commute with the total spin operator \( S_t \). As a result, the Hamiltonian becomes block diagonal in terms of relatively small (\( O(N) \)) Hilbert-space sectors. The energy levels and properties within each sector depend on the total spin \( s_t \), which can take values from \( 0 \) to \( N/2 \) (assuming \( N \) is even). The Hilbert space dimension in each \( s_t \) sector is \( 2s_t + 1 \). The number of copies of the spin \( s_t \) sector is the number of ways \( N \) spin-\(\frac{1}{2}\) objects can be combined into a total spin \( s_t \). This multiplicity \( d(s_t) \) is one for \( s_t = N/2 \), and for \( s_t < N/2 \), it can be expressed in terms of the combinatorial factor \( C_{N,s_t} \) as:  
\begin{equation}
    d(s_t) = \binom{N}{\frac{N}{2} + s_t} - \binom{N}{\frac{N}{2} + s_t + 1}.
\end{equation}  
Therefore, instead of dealing with an exponentially large Hilbert space of size \( 2^N \), we only need to diagonalize matrices of size \( 2s_t + 1 \) within each total spin sector, which is much smaller. The full Hilbert space dimension is then effectively reduced to:
\begin{equation}
    \mathcal{D}_{\text{reduced}} = \sum_{S_t = 0}^{N/2} (2s_t + 1) d(s_t).
\end{equation}
This reduction makes it possible to study systems with thousands of spins, which would otherwise be computationally intractable.

In this case, the electronic spin couples to the nuclear spin through an additional term in the Hamiltonian. Since the nuclear spin introduces an additional degree of freedom, the total nuclear spin also becomes a conserved quantity. Therefore, the total nuclear spin $m$ can take values from \( -N/2 \) to \( N/2 \). The Hilbert space dimension for a given nuclear spin sector is \( m+1 \). The number of different nuclear spin sectors is determined by the combinatorial factor:
\begin{equation}
    d(m) = \binom{N}{\frac{N}{2}+m}.
\end{equation}
Thus, the total Hilbert space dimension in a combined electronic and nuclear spin sector with total spin \( s_t \) and nuclear spin \( m \) becomes:
\begin{equation}
    D(m,s_t) = \sum_{m=-N/2}^{N/2}d(m)(m+1)\sum_{s_t = 0}^{N/2} d(s_t)(2s_t + 1).
\end{equation}

%%%%%%%%%%%%%%%%%%%%%%%%%%%%%%%%%%%%%%%%%%%%%%%%%%%%%%
\section{\label{SM3}Mean field analysis with finite transverse field}
We consider the effect of nuclear coupling on the phase boundary shift to leading order in \( A \). The starting Hamiltonian is given by 
\begin{equation}
    \mathcal{H} = \mathcal{H}_0 + 4A \sum_i I_i^z \frac{S^x_t}{N},
\end{equation}
where \( A \) is the nuclear coupling constant, \( S^x_t = \sum_i S_i^x \) is the total electronic spin in the \( x \)-direction, and \( I_i^z \) is the nuclear spin operator. To a good approximation, we employ the mean-field approximation, where each nuclear spin experiences a field due to the electronic spin:
\begin{equation}
    h_{\text{nuc}} = 4A \langle S_i^x \rangle \quad \text{with} \quad \langle S_i^x \rangle = \frac{\langle S^x_t \rangle}{N}.
\end{equation}
Using the mean-field approximation, the expectation value of the electronic spin in the \( x \)-direction is given by
\begin{equation}
    \langle S_i^x \rangle = \frac{1}{2} \tanh \left( \frac{T_Q}{T} \frac{h_x}{h_c^0} \right),
\end{equation}
where $T_Q = T_c (h_T=0)$ and $h_c^0$ are mentioned in the main text. Therefore, the nuclear field becomes
\begin{equation}
    h_{\text{nuc}}(T, h_x) = - 2A \tanh \left( \frac{T_Q}{T} \frac{h_x}{h_c^0} \right).
\end{equation}
This causes a nuclear polarization, which is given by
\begin{equation}
    \langle I_i^z \rangle = -\frac{1}{2} \tanh \frac{\beta h_{\text{nuc}}}{2} 
    = -\frac{1}{2} \tanh \left\{ \beta A \tanh \left( \frac{T_c}{T} \frac{h_x}{h_c} \right) \right\}.
\end{equation}
With this polarization, the effective Hamiltonian becomes
\begin{equation}
    \mathcal{H} = \mathcal{H}_0 - 2A \tanh \left\{ \beta A \tanh \left( \frac{T_Q}{T} \frac{h_x}{h_c^0} \right) \right\} S^x_t.
\end{equation}
Thus, the electrons effectively experience a modified transverse field given by
\begin{equation}
    h_x + 2A \tanh \left\{ \beta A \tanh \left( \frac{T_Q}{T} \frac{h_x}{h_c^0} \right) \right\}.
\end{equation}
This modified field captures the leading-order shift in the phase boundary due to the coupling between the electronic and nuclear spins.
The phase boundary must be shifted from the \( A = 0 \) calculation by the amount
\begin{equation}
    \Delta h_x = -2A \tanh \left( \beta A \tanh \left( \frac{T_Q}{T} \frac{h_x}{h_c^0} \right) \right).
\end{equation}
If we numerically evaluate the phase boundary using the relation
\begin{equation}
    T_c(h_x) = T_Q \frac{h_x/h_c^0}{\tanh^{-1}(h_x/J_z)},
\end{equation}\
it provides a pair of points at the phase boundary \((h_x, T)\). 
Therefore, the shifted phase boundary should be given by
\begin{equation}
    (h_x - \Delta h_x, T).
\end{equation}
By setting \( T_Q = h_c^0 = J_z = 1 \), the shift in the phase boundary simplifies to
\begin{equation}
    \Delta h_x = -2A \tanh \left( \frac{A}{T} \tanh \left( \frac{h_x}{T} \right) \right).
\end{equation}

\section{\label{SM4}Finite-size scaling of the excitation gap near the critical point}
To further characterize the critical behavior of the model, we analyze the finite-size scaling of the low-energy excitation gap in the vicinity of the critical transverse field $h_x \approx 0.99$. In the ordered phase the ground state is expected to be doubly degenerate in the thermodynamic limit. For finite system sizes this degeneracy is slightly lifted, which leads to a small gap between the two lowest-energy states.

Deep in the ordered phase the excitation gap is extremely small and decreases rapidly with increasing system size, consistent with the expected double degeneracy of the ground state in the thermodynamic limit. However, as the transverse field approaches the critical point, the degeneracy is lifted and a small but finite gap opens.

To quantify this behavior we perform a finite-size scaling analysis of the excitation gap $\Delta$ as a function of the inverse system size $1/N$. The numerical data are well described by a power-law scaling form

\begin{equation}
\Delta(N) \sim N^{-\alpha},
\end{equation}

where $\alpha$ is the effective finite-size scaling exponent.

Exactly at the critical point the excitation gap is expected to follow a characteristic power-law scaling. Our numerical results show that the exponent approaches $\alpha \approx \frac{1}{3}$, which signals the critical scaling regime of the model.

Fig.\ref{fig:gap_scaling} show representative finite-size scaling plots of the excitation gap for several transverse field values near the critical point. The dashed lines represent power-law fits used to extract the exponent $\alpha$. As the transverse field approaches $h_x \approx 0.99$, the extracted exponent becomes close to $1/3$. Moving away from the critical point toward the ordered phase the exponent increases, reflecting the rapid collapse of the excitation gap due to the emergent ground-state degeneracy.

\begin{table}[h]
\caption{Finite-size scaling exponent $\alpha$ of the excitation gap near the critical point. The exponent approaches $\alpha \approx 1/3$ near $h_x \approx 0.99$, indicating the critical scaling regime.}
\begin{ruledtabular}
\begin{tabular}{cc}
$h_x$ & $\alpha$ \\
\hline
0.989 & 0.52 \\
0.990 & 0.33 \\
0.991 & 0.23 \\
0.992 & 0.17 \\
0.993 & 0.13 \\
0.994 & 0.11 \\
\end{tabular}
\end{ruledtabular}
\label{tab:gap_scaling}
\end{table}

\begin{figure*}[t]
\centering
\includegraphics[width=0.32\textwidth]{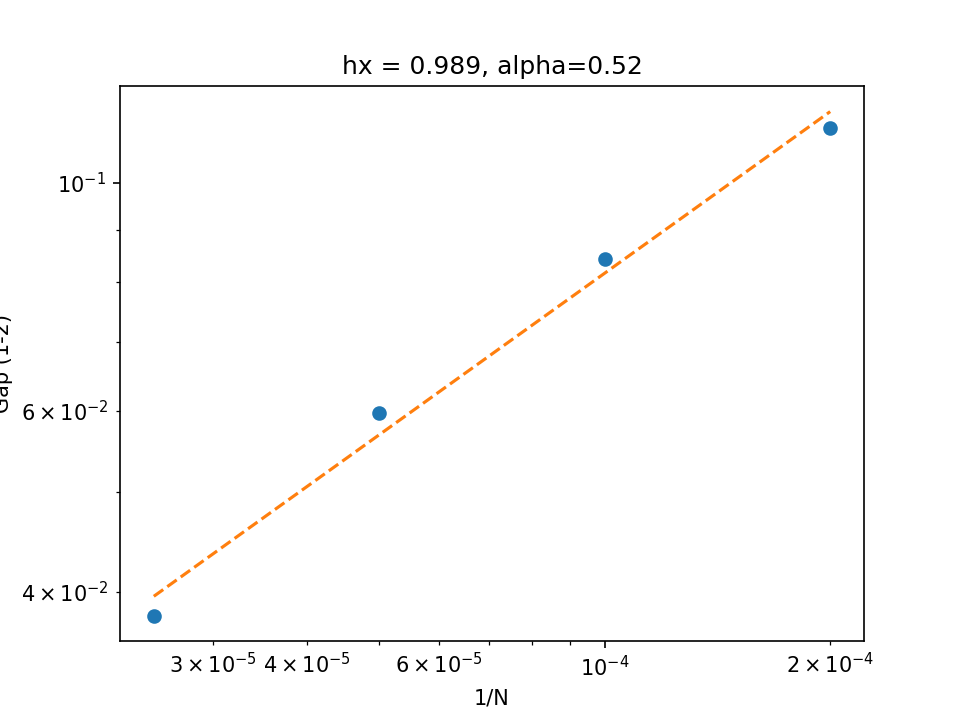}
\includegraphics[width=0.32\textwidth]{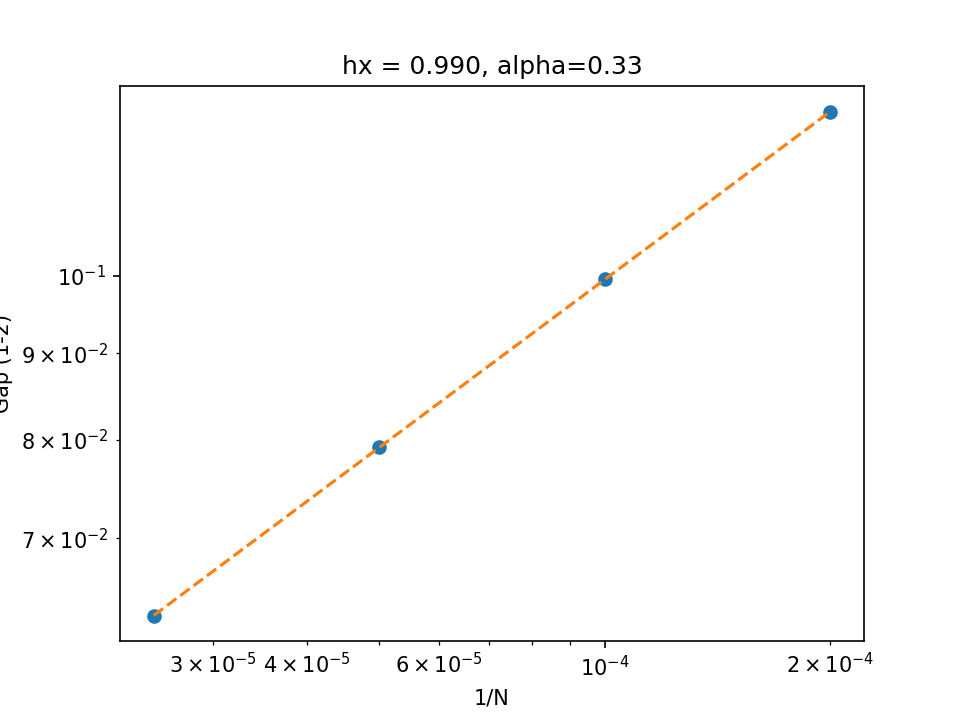}
\includegraphics[width=0.32\textwidth]{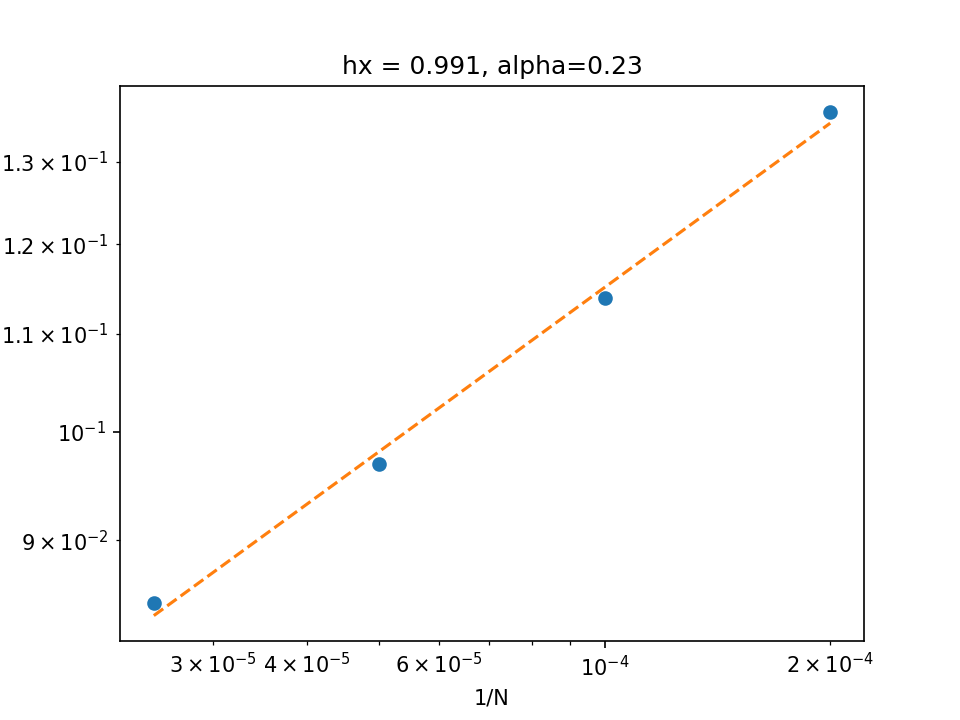}

\vspace{0.2cm}

\includegraphics[width=0.32\textwidth]{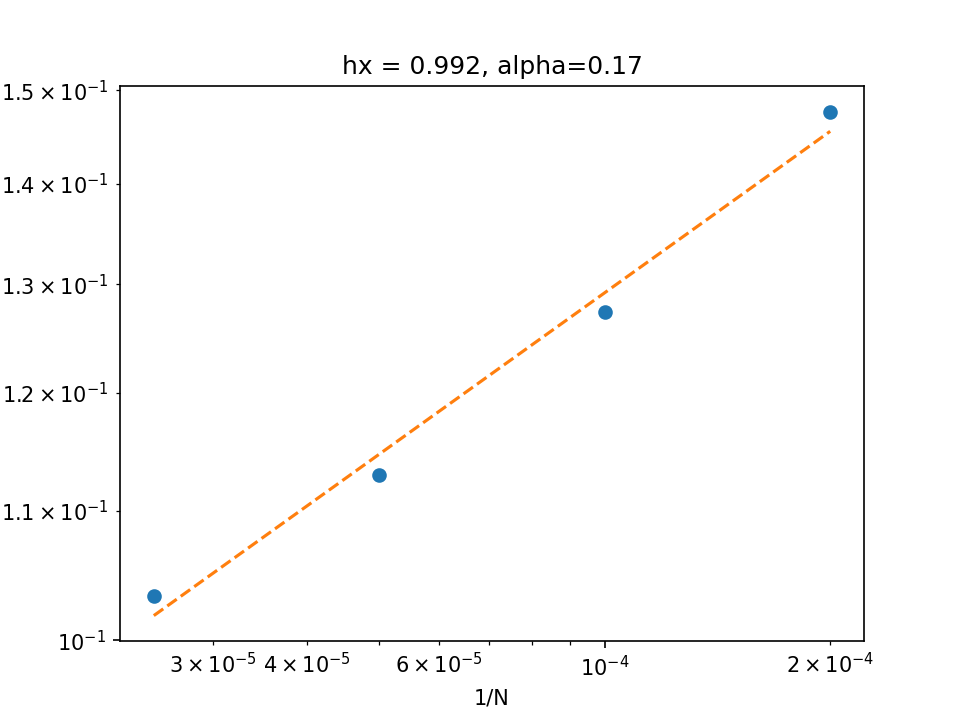}
\includegraphics[width=0.32\textwidth]{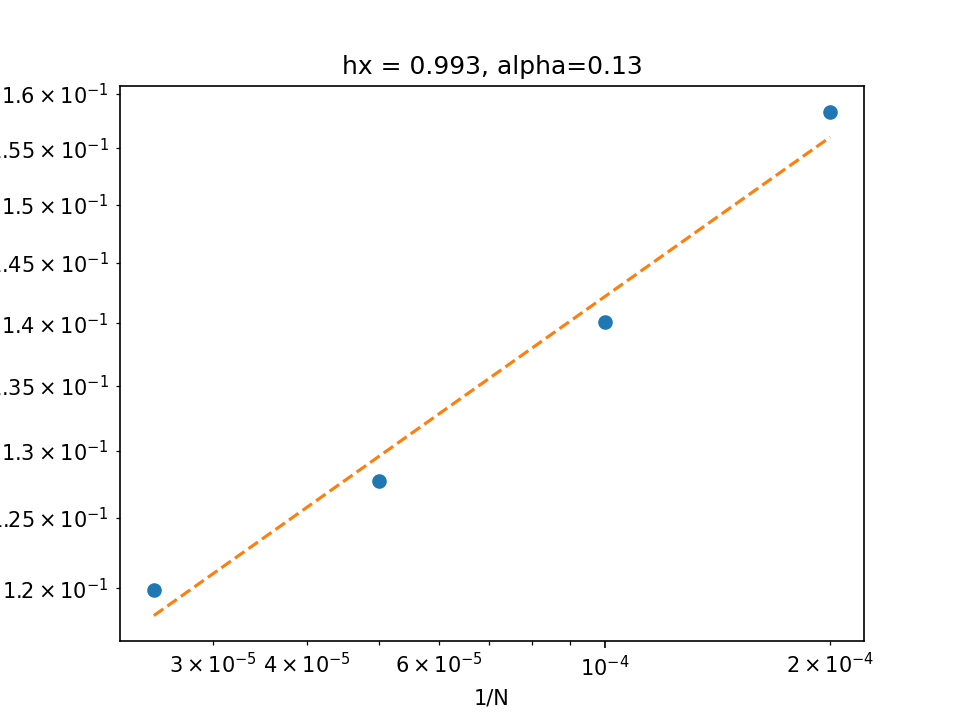}
\includegraphics[width=0.32\textwidth]{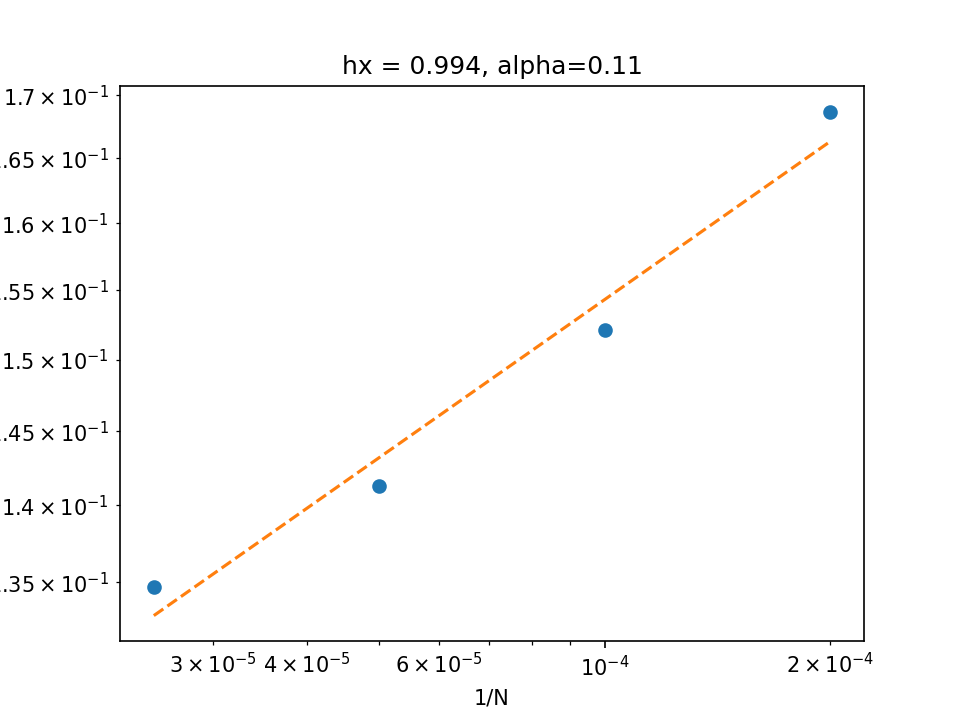}

\caption{Finite-size scaling of the excitation gap $\Delta$ as a function of $1/N$ for several transverse field values near the critical point. The dashed lines represent power-law fits used to extract the scaling exponent $\alpha$. The exponent approaches $\alpha \approx 1/3$ near $h_x \approx 0.99$, indicating the critical scaling regime.}
\label{fig:gap_scaling}
\end{figure*}

\bibliography{ref}
\bibliographystyle{apsrev4-2}
\end{document}
